# Supplementary material for: Stabilizing a high-pressure phase in InSb at ambient conditions with a laser-driven pressure pulse
Source: arXiv:1712.05370 source file (2017-12-14)
Supplement: Supplementary file 1 [file InSb_SM.pdf]

# Supplemental Material for Stabilizing a high-pressure phase in InSb at ambient conditions with a laser-driven pressure pulse

A. Jarnac,[1,2] Xiaocui Wang,[2] Å. U. J Bengtsson,[2] M. Burza,[1] J. C. Ekström,[2] H. Enquist,[1] A. Jurgilaitis,[1] N. Kretzschmar,[3] A. I. H. Persson,[2] C. M. Tu,[2] M. Wulff,[3] F. Dorchies,[4] and J. Larsson[1,2]

[1]*MAX IV Laboratory, Lund University, P.O. Box 118, SE-221 00 Lund, Sweden*

[2]*Department of Physics, Lund University, P.O. Box 118, SE-221 00 Lund, Sweden*

[3]*ESRF The European Synchrotron, 71 Avenue des Martyrs, 38000 Grenoble, France*

[4]*Univ. Bordeaux, CNRS, CEA, CELIA (Centre Lasers Intenses et Applications), UMR 5107, 33400 Talence, France*

(Dated: December 6, 2017)

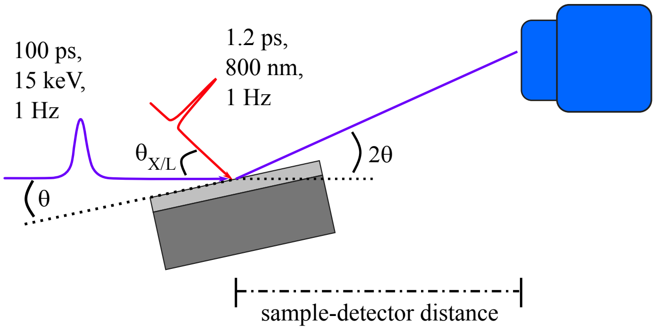


Figure 1. Sketch of the experimental setup at ID09 (ESRF). X-rays were incident at an angle $\theta$ with respect to the sample surface. We illuminated the sample with an 800 nm laser pulse. The angle $\theta_{X/L}$ between X-rays and the laser was set to 10°. The X-ray diffracted intensity was recorded by the rayonix MX-170 HS detector at a distance of 200 mm from the sample.

## EXPERIMENTAL METHODS

A sketch of the experimental setup is shown in figure 1. To maximize the laser absorption in the Al film, we set the laser angle of incidence close to the Brewster angle. As a result, the laser beam was nearly co-propagating with X-rays and the angle $\theta_{X/L}$ between them was set to 10°. We performed X-ray measurements at two different angles of incidence $\theta$. Firstly, *time-resolved* X-ray diffraction was performed for a set of angle $\theta$ around the Bragg angle of the InSb (111) reflection ($\theta_B = 6.35°$). We acquired $\theta$ - $2\theta$ diffraction curve in order to probe the strain along the [111] direction. Secondly, *in situ* X-ray diffraction was performed at $\theta = 1.3°$ and the full diffraction pattern was recorded in order to find evidences for the InSb-III phase. When rotating the sample from $\theta = 6.3$ to 1.3°, the projection of the laser spot increase by 40%. We kept the fluence constant for the two angles of incidence, and this was verified by measuring the post mortem damage size, where the size increased by 40%. In both measurements, we recorded the X-ray diffracted from the sample by using the rayonix MX-170 HS detector (170 mm × 170 mm) at a distance of 200 mm from the sample.

## TRANSIENT NATURE OF THE PRESSURE PULSE

The simulations predict a traveling ultrashort pressure pulse. We verified this effect by acquiring the X-ray reflectivity at $\theta = 6.85°$ as a function of the delay between the laser pulse

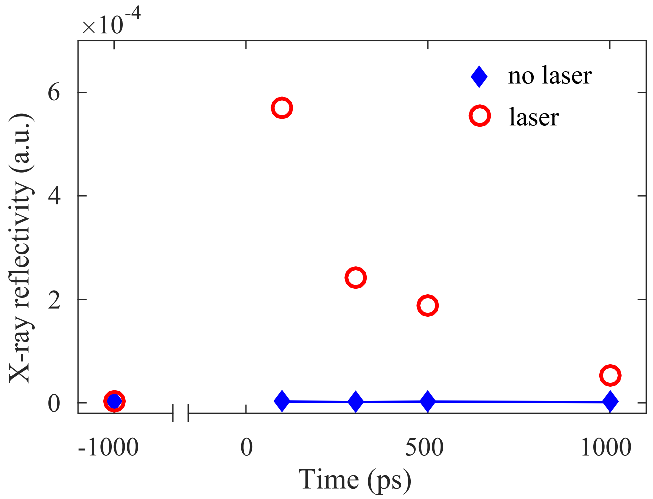


Figure 2. Time-dependence of the X-ray reflectivity at an angle $\theta$ of 6.85°. The time-evolution of the X-ray reflectivity is consistent with 3900 m/s propagation velocity in InSb [1] and a probe depth of 2300 nm for 15 keV X-rays [2].

and the X-ray pulse (Fig. 2). It can be seen that the X-ray reflexivity follows a decaying exponential with a width of $\sim$ 500 ps (1/e). This time scale is consistent with 3900 m/s propagation velocity in InSb [1] and a probe depth of 2300 nm for 15 keV X-rays [2]. To ensure the absence of strain before the laser interaction with the Al film, we also recorded one data point where the X-ray pulse was 1 ns in advance compare to the laser pulse.

[1] L. J. Slutsky and C. W. Garland, Phys. Rev. **113**, 167 (1959).

[2] B. Henke, E. Gullikson, and J. Davis, Atomic Data and Nuclear Data Tables **54**, 181 (1993).
